# Supplementary material for: Multi-modal Instruction Tuned LLMs with Fine-grained Visual Perception
Source: arXiv:2403.02969 source file (2024-03-25)
Supplement: Supplementary file 1 [file X_suppl.tex]

\clearpage
\setcounter{page}{1}
\maketitlesupplementary

% \section{Rationale}
% \label{sec:rationale}
% % 
% Having the supplementary compiled together with the main paper means that:
% % 
% \begin{itemize}
% \item The supplementary can back-reference sections of the main paper, for example, we can refer to \cref{sec:intro};
% \item The main paper can forward reference sub-sections within the supplementary explicitly (e.g. referring to a particular experiment); 
% \item When submitted to arXiv, the supplementary will already included at the end of the paper.
% \end{itemize}
% % 
% To split the supplementary pages from the main paper, you can use \href{https://support.apple.com/en-ca/guide/preview/prvw11793/mac#:~:text=Delete%20a%20page%20from%20a,or%20choose%20Edit%20%3E%20Delete).}{Preview (on macOS)}, \href{https://www.adobe.com/acrobat/how-to/delete-pages-from-pdf.html#:~:text=Choose%20%E2%80%9CTools%E2%80%9D%20%3E%20%E2%80%9COrganize,or%20pages%20from%20the%20file.}{Adobe Acrobat} (on all OSs), as well as \href{https://superuser.com/questions/517986/is-it-possible-to-delete-some-pages-of-a-pdf-document}{command line tools}.

\section{Implementation Details}

\subsection{Network Architecture}

The base MLLM of {\textbf{AnyRef}} is based on LLaVA-7B-v1-1, where we freeze the image encoder and visual-language projection layer, and train the LLM using LoRA\cite{hu2021lora}.
% \footnote{\url{https://github.com/haotian-liu/LLaVA/blob/main/docs/MODEL_ZOO.md}}
For audio input, we adopt the pre-trained audio encoder from ImageBind-H \cite{girdhar2023imagebind}, which is also frozen during fine-tuning.
% \footnote{\url{https://github.com/facebookresearch/ImageBind}}
The audio-language projection layer, akin to the visual-language projection layer, comprises a single trainable MLP layer.
The adopted segmentation model is SAM-H \cite{kirillov2023segany}, featuring a frozen image encoder and a trainable mask decoder.
% \footnote{\url{https://github.com/facebookresearch/segment-anything}}
In line with \cite{lai2023lisa}, we utilize a 2-layer MLP to map the mask embedding to the input of the mask decoder.

\subsection{Instruction Formulation}

In contrast to LISA\cite{lai2023lisa}, {\textbf{AnyRef}} is required to generate textual descriptions along with masks.
Hence, we must create supplementary question-answer templates distinct from LISA's, which primarily uses answer templates such as ``{\texttt{It is {\textless{\texttt{SEG}}\textgreater}}}" or ``{\texttt{Sure, it is {\textless{\texttt{SEG}}\textgreater}}}".
Additionally, owing to the introduced \emph{Refocusing Mechanism} (as detailed in \cref{refocusing}), tokens preceding the {\textless{\texttt{obj}}\textgreater} token are intended to offer textual guidance, while the phrase ``{\texttt{it is}}" does not cover any meaningful information.

For textural referring segmentation datasets (including general semantic/instance segmentation and referring expression segmentation), the question template is ``\texttt{Can you segment \{exp\} in this image?}", where \texttt{\{exp\}} represents either the textural class name or the description.
And the answer is ``\texttt{\{exp\} \textless{\texttt{obj}}\textgreater.}", indicating that {\textbf{AnyRef}} needs to repeat the grounding description to offer textural guidance for the {\textless{\texttt{obj}}\textgreater} token, as part of the \emph{Refocusing Mechanism}.
We apply the same approach for image-level referring and audio-visual samples, replacing \texttt{\{exp\}} with the textural target class name."

\subsection{Human Evaluation on Referring Expression Generation}

We follow previous work \cite{ye2023ireg} to conduct human evaluation on generated referring expressions.
We randomly sample 100 images with corresponded bounding boxes for each test split, and generate textural expressions using different models.
The images, along with the bounding boxes and the generated referring expressions, are presented to five different evaluators.
They assess whether the target object could be unambiguously identified based on the provided referring expression; if so, the referring expression is labelled as correct.
% The image with bounding-box of the target object and generated
% RE are displayed to five different evaluator to judge whether the target object can be located dis-ambiguously according to the referring expression.

\section{Qualitative Results}

We provide additional visualizations for all feasible tasks within the {\textbf{AnyRef}}, including referring expression segmentation, image-referring segmentation, audio-visual segmentation and region-level referring expression generation.
The results are produced from the same general model, without fine-tuning on each single task.

In \cref{fig:ref}, we show the referring segmentation results from textural descriptions, comparing the ground-truth, the concurrent model LISA \cite{lai2023lisa} and {\textbf{AnyRef}}.
% \footnote{\url{https://github.com/dvlab-research/LISA}}
In comparison to LISA, our {\textbf{AnyRef}} excels in identifying the correct referring object and generated more accurate masks corresponding to the ground-truth (\emph{e.g.}, in the 2nd and 5th rows, accurate mask shapes of the urn and giraffe were detected without including the background).

In \cref{fig:img_ref} and \cref{fig:img_ref_mask}, we present the image-level referring segmentation results without and with corresponding mask annotations.
When lacking explicit mask annotations, {\textbf{AnyRef}} demonstrates the capability to comprehend image references and identify similar objects or regions within the queried image.
With the inclusion of mask annotations, background noise is eliminated, resulting in clearer identification of referring objects (\emph{e.g.}, in the last row of \cref{fig:img_ref_mask}, {\textbf{AnyRef}} accurately identifies trains solely from the train door), which enhances object recognition and reduces ambiguity.
Unlike \cite{luddecke2022imagetextprompt}, which utilizes visual prompt engineering (\emph{e.g.}, adjusting background intensity, blurring, or adding outlines) to emphasize objects, we found that using a black background performs adequately in our scenarios. 
Therefore, we opt not to include additional visual prompting in the image references to maintain simplicity.

In \cref{fig:avs}, we show the audio-visual segmentation results on AVSBench \cite{zhou2022avs}.
Compared with ground-truth mask annotations, {\textbf{AnyRef}} is able to produce more precises masks.

In \cref{fig:ref_inv}, we show the region-level referring expression generation results between {\textbf{AnyRef}} and two recent region-aware LMMs, Shikra \cite{chen2023shikra} and KOSMOS-2 \cite{peng2023kosmos}.
% \footnote{\url{https://github.com/shikras/shikra}}
% \footnote{\url{https://github.com/microsoft/unilm/tree/master/kosmos-2}}
Thank to the powerful LLM pre-trained from vision instructions (where {\textbf{AnyRef}} is initialized from \cite{liu2023llava}), we suprisingly found that it still keeps the OCR ability (\emph{e.g.}, it correctly recognizes ``Happy halloween" on the shirt in the last row of \cref{fig:ref_inv}).
Moreover, {\textbf{AnyRef}} has the capability to generate grounding masks corresponding to bounding boxes simultaneously, towards more fine-grained object perceptions.

\section{Discussions}

We further investigate whether using multiple references from different modalities improves performances, \emph{e.g.}, providing textural descriptions and audio inputs or image-level references simultaneously.
The prompt is built like: ``\texttt{Can you segment \{exp\} with sound of {\textless{\texttt{aud\_ref}}\textgreater}{\textless{\texttt{aud\_feat}}\textgreater}{\textless{\texttt{/aud\_ref}}\textgreater} in this image?}"
However, we obverse no performance improvement.
% We speculate that due to the LLM's robust understanding and reasoning abilities, as well as its capacity for multi-modal feature alignments, it can transfer prompts from different modalities into the textural space.
We speculate that due to the LLM's robust understanding and reasoning abilities, alongside its capacity for multi-modal feature alignments, it has the capability to transfer prompts from various modalities into the textual space.
% Therefore, prompting the same concepts repeatedly will not boost its performance but potentially confuse the LLM.
Therefore, repeatedly prompting the same concepts may not enhance its performance but could potentially confuse the LLM."
% However, this is still an explored area which needs further investigation, which beyond the scope of this paper, and we hope to dig more in the future.
However, this area remains relatively unexplored and requires further investigation, which goes beyond the scope of this paper. We hope to delve deeper into it in future research.

\begin{figure*}[tbp]
    \centering
    \includegraphics[width=0.95\textwidth]{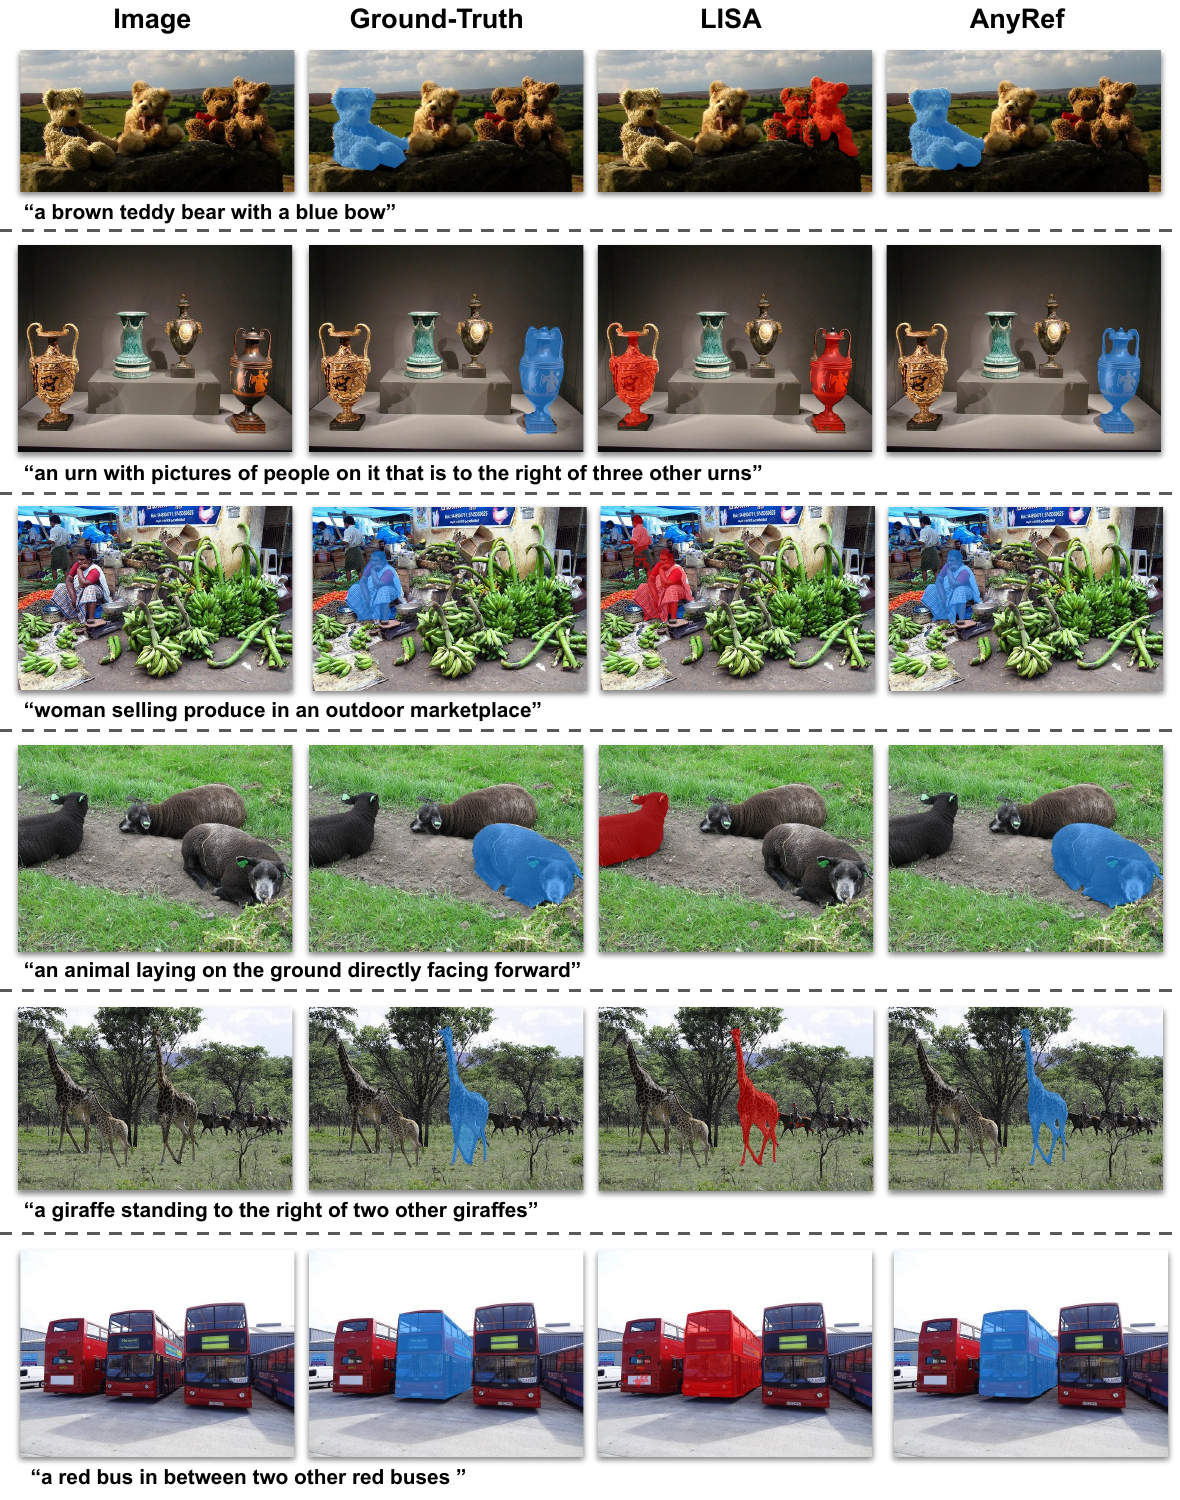}
    \caption{Qualitative results of {\textbf{Referring Expression Segmentation}}. The text below indicates the textural referring expression. LISA \cite{lai2023lisa} occasionally fails to identify the correct referring object, whereas {\textbf{AnyRef}} can produce more precise masks compared to the ground-truth (\emph{e.g.}, urn in the 2nd row and giraffe in the 5th row).}
    \label{fig:ref}
\end{figure*}

\begin{figure*}[tbp]
    \centering
    \includegraphics[width=\textwidth]{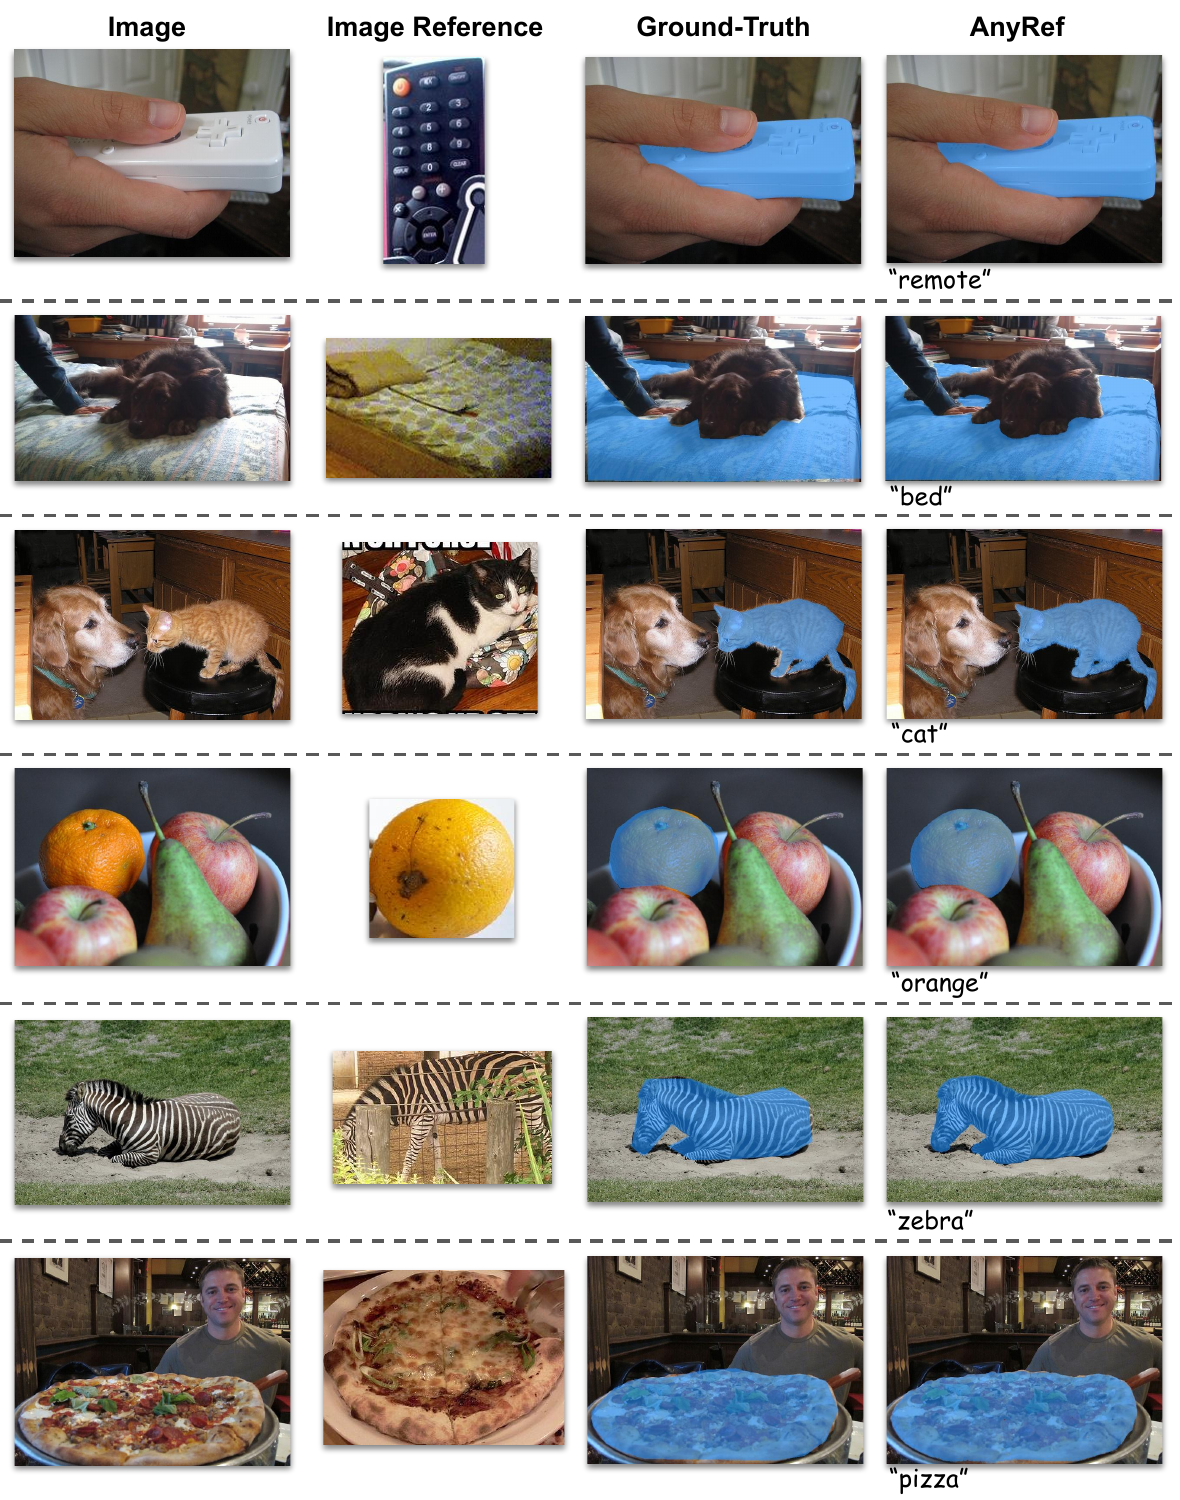}
    \caption{Qualitative results of {\textbf{Image Referring Segmentation}}.}
    \label{fig:img_ref}
\end{figure*}

\begin{figure*}[tbp]
    \centering
    \includegraphics[width=\textwidth]{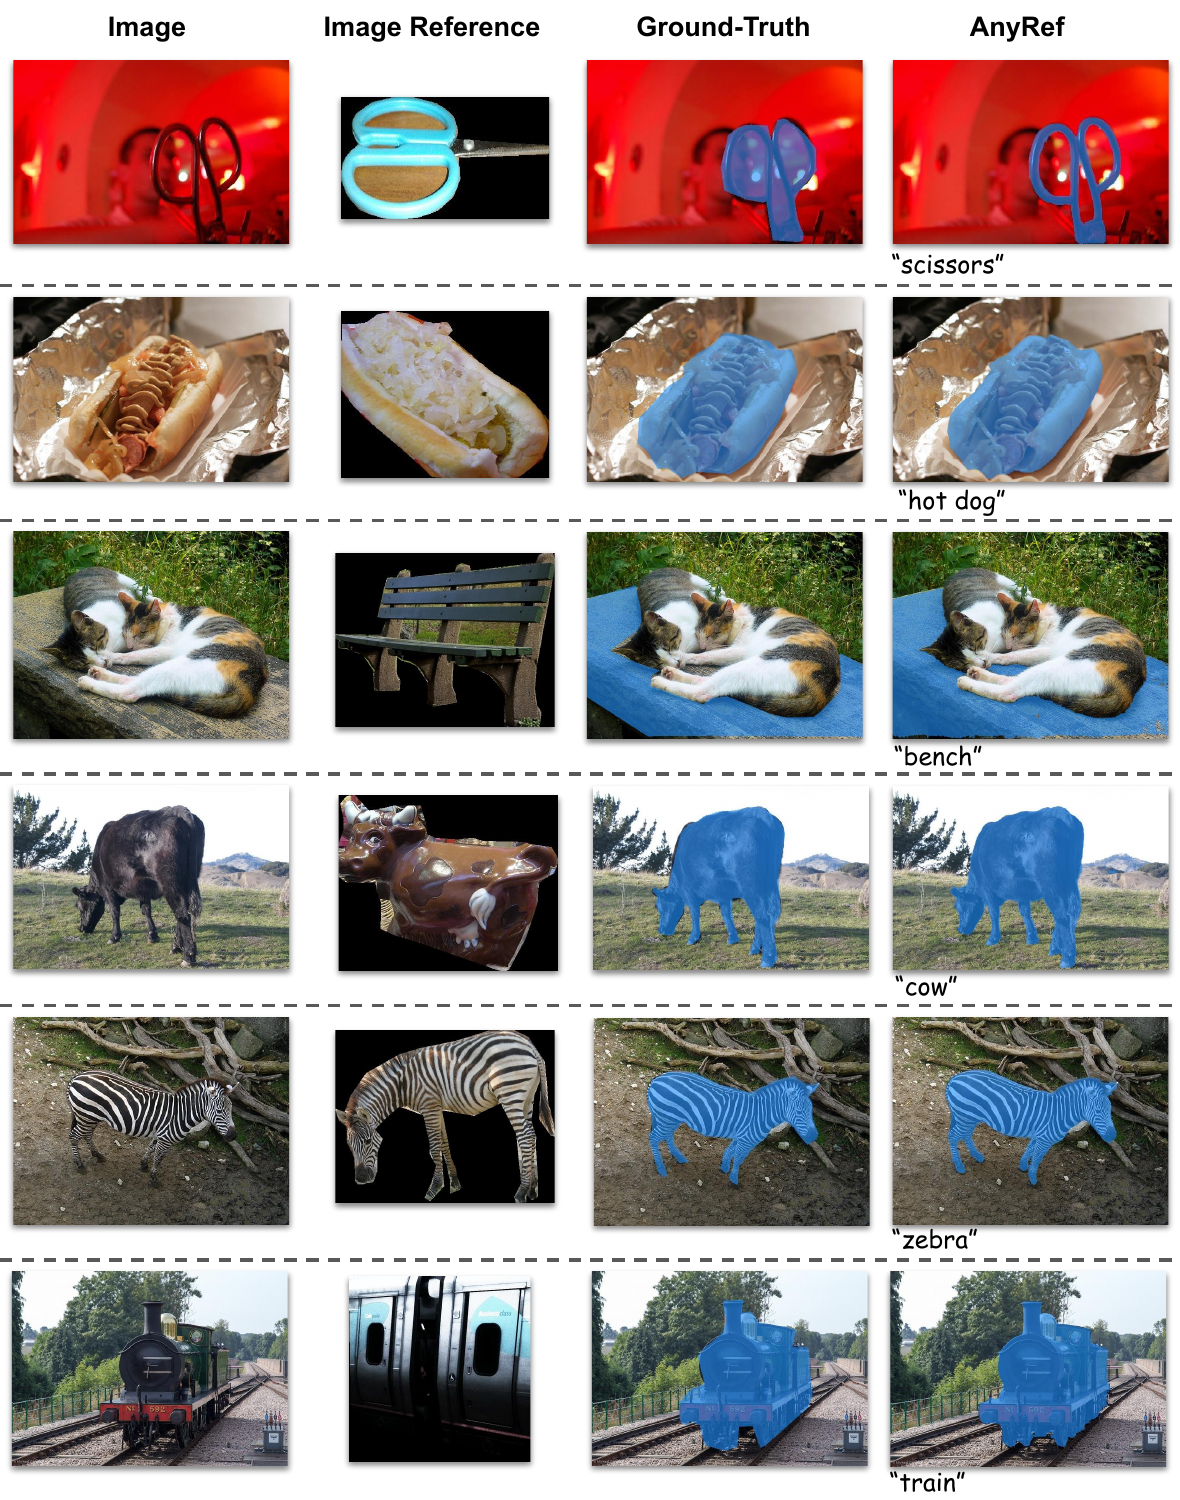}
    \caption{Qualitative results of {\textbf{Image Referring Segmentation with masks}}.}
    \label{fig:img_ref_mask}
\end{figure*}

\begin{figure*}[tbp]
    \centering
    \includegraphics[width=\textwidth]{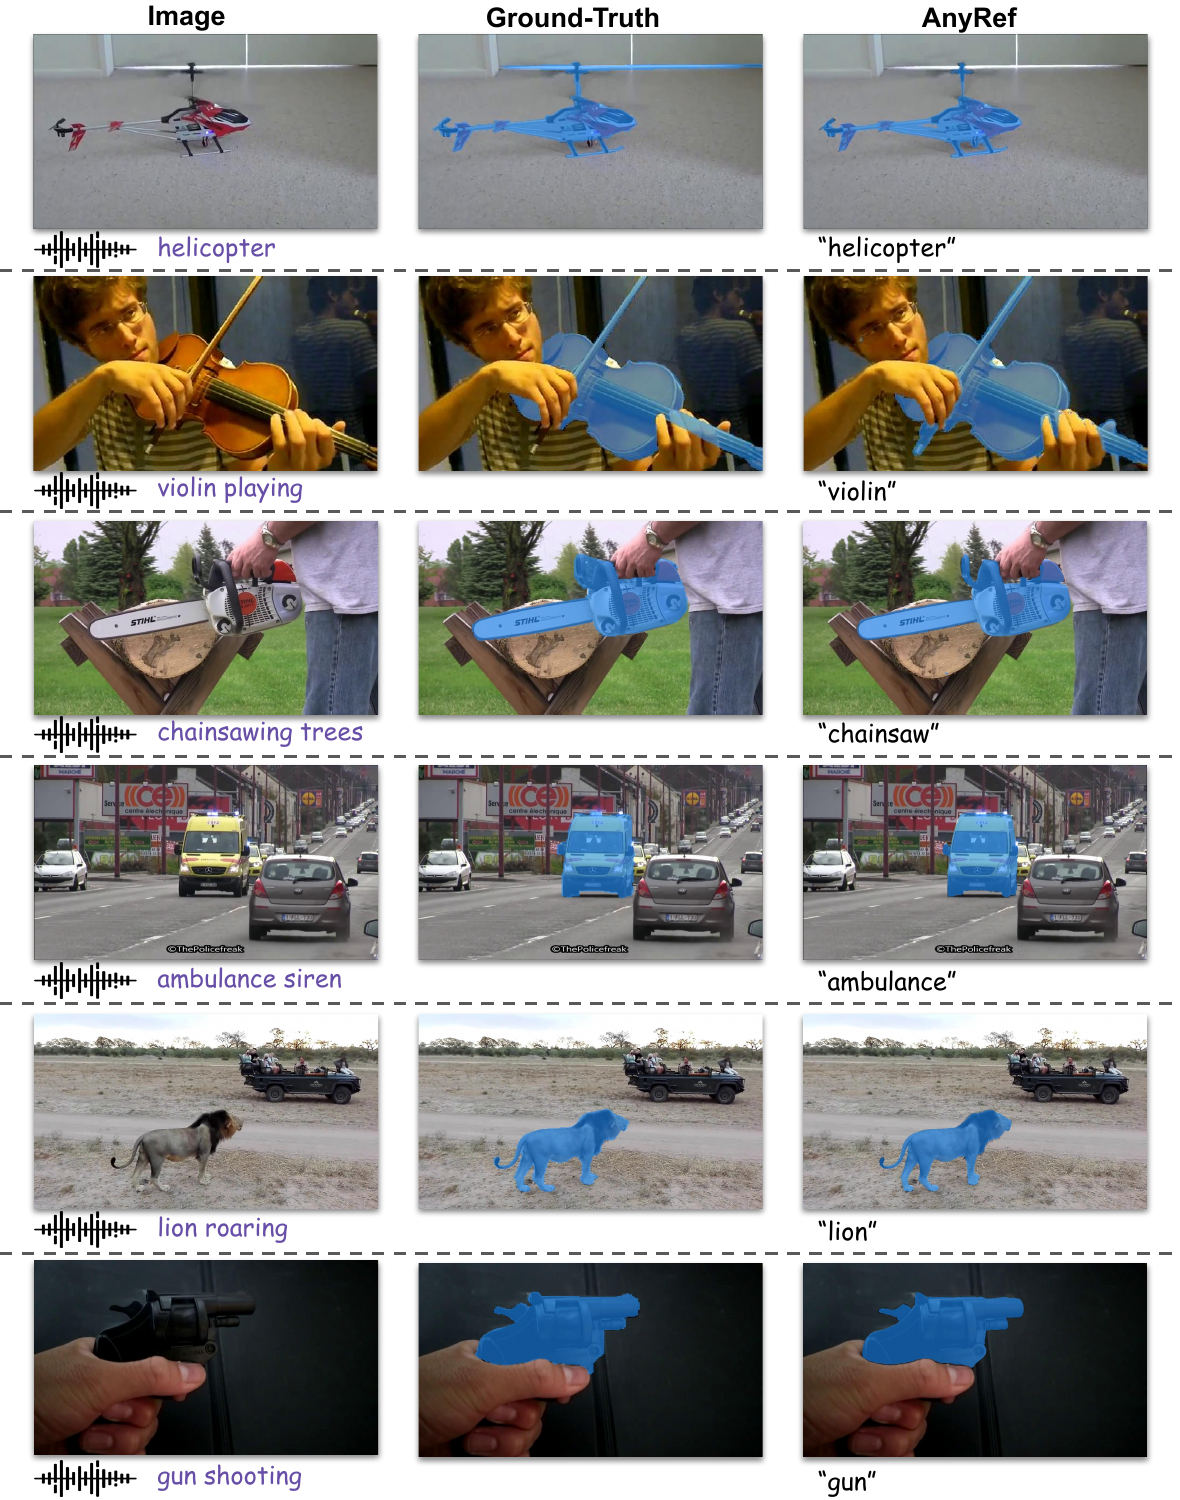}
    \caption{Qualitative results of {\textbf{Audio-Visual Segmentation}}. Furthermore, {\textbf{AnyRef}} can also generate textual class name of the target sounding object based on the audio input.}
    \label{fig:avs}
\end{figure*}

\begin{figure*}[tbp]
    \centering
    \includegraphics[width=0.95\textwidth]{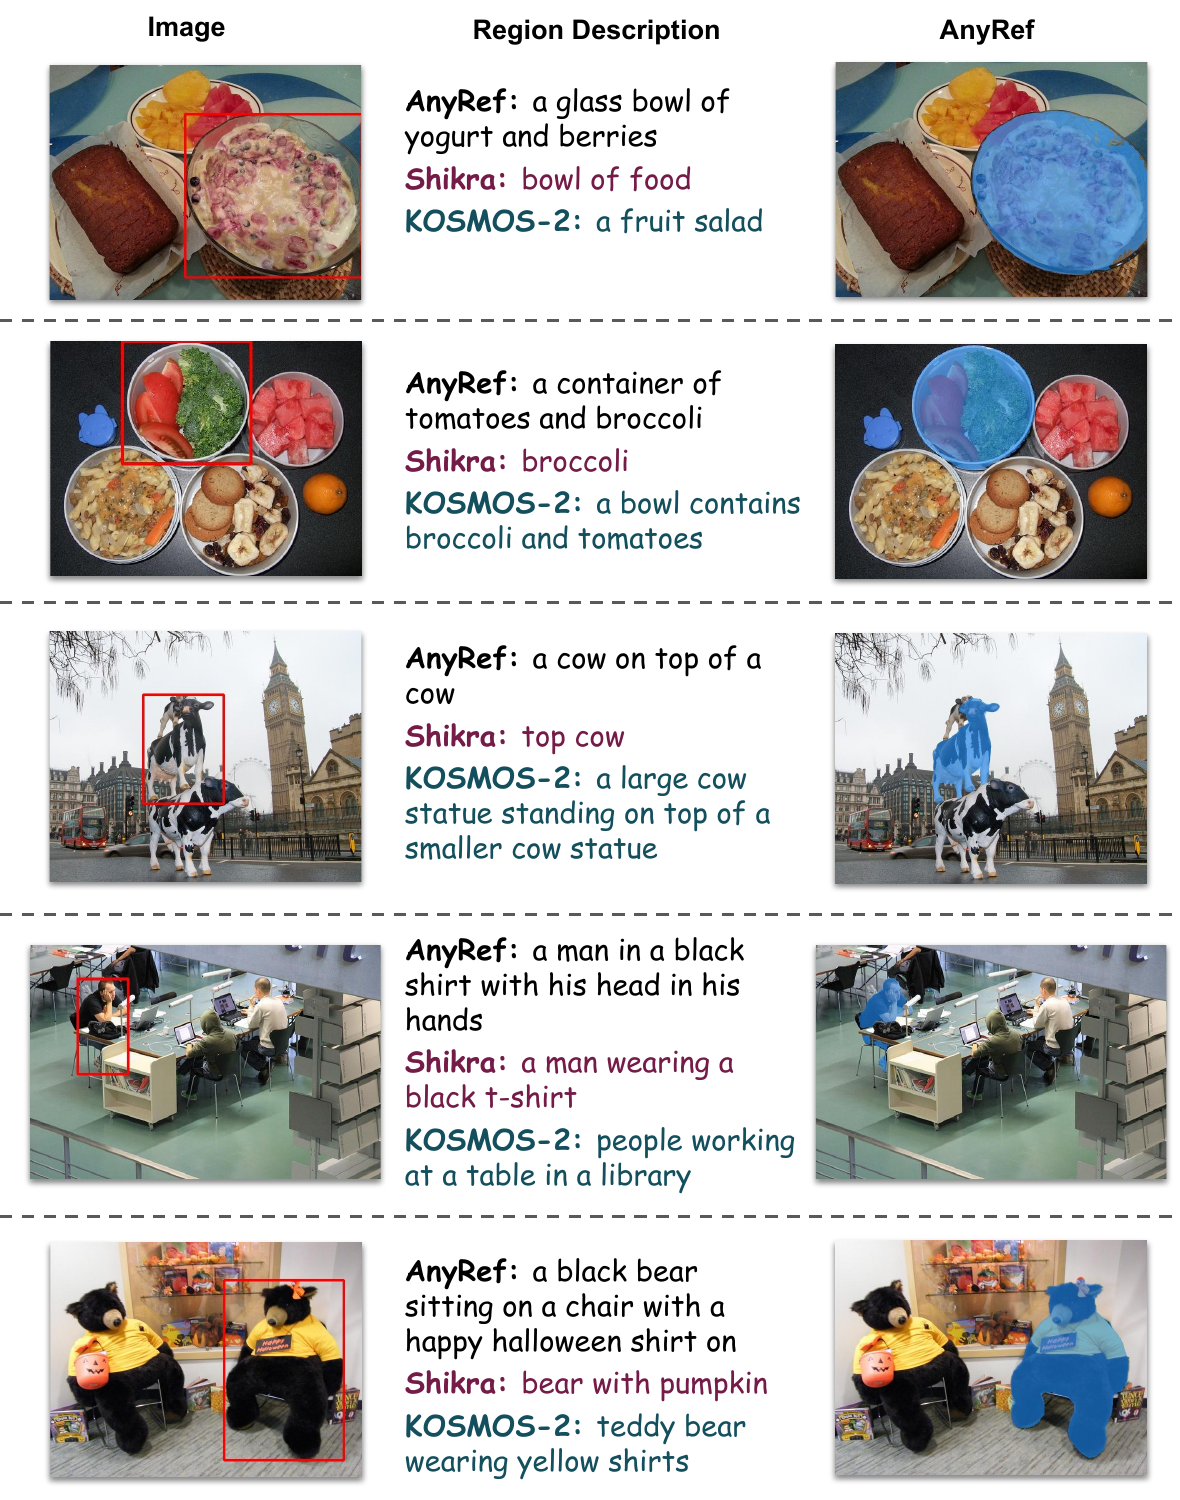}
    \caption{Qualitative results of {\textbf{Region-level Referring Expression Generation}} compared with Shikra \cite{chen2023shikra} and KOSMOS-2 \cite{peng2023kosmos}. {\textbf{AnyRef}} is initialized from LLaVA \cite{liu2023llava}, so it still keeps the OCR ability (\emph{e.g.}, it recognizes ``happy halloween" on the shirt). Additionally, {\textbf{AnyRef}} can also output the grounding mask corresponding to the bounding-box.}
    \label{fig:ref_inv}
\end{figure*}
